# Supplementary material for: UltraMNIST Classification: A Benchmark to Train CNNs for Very Large Images
Source: arXiv:2206.12681 source file (2022-06-25)
Supplement: Supplementary file 1 [file appendix.tex]

% \begin{figure}
%     \centering
%     \includegraphics[width=\linewidth]{neurips/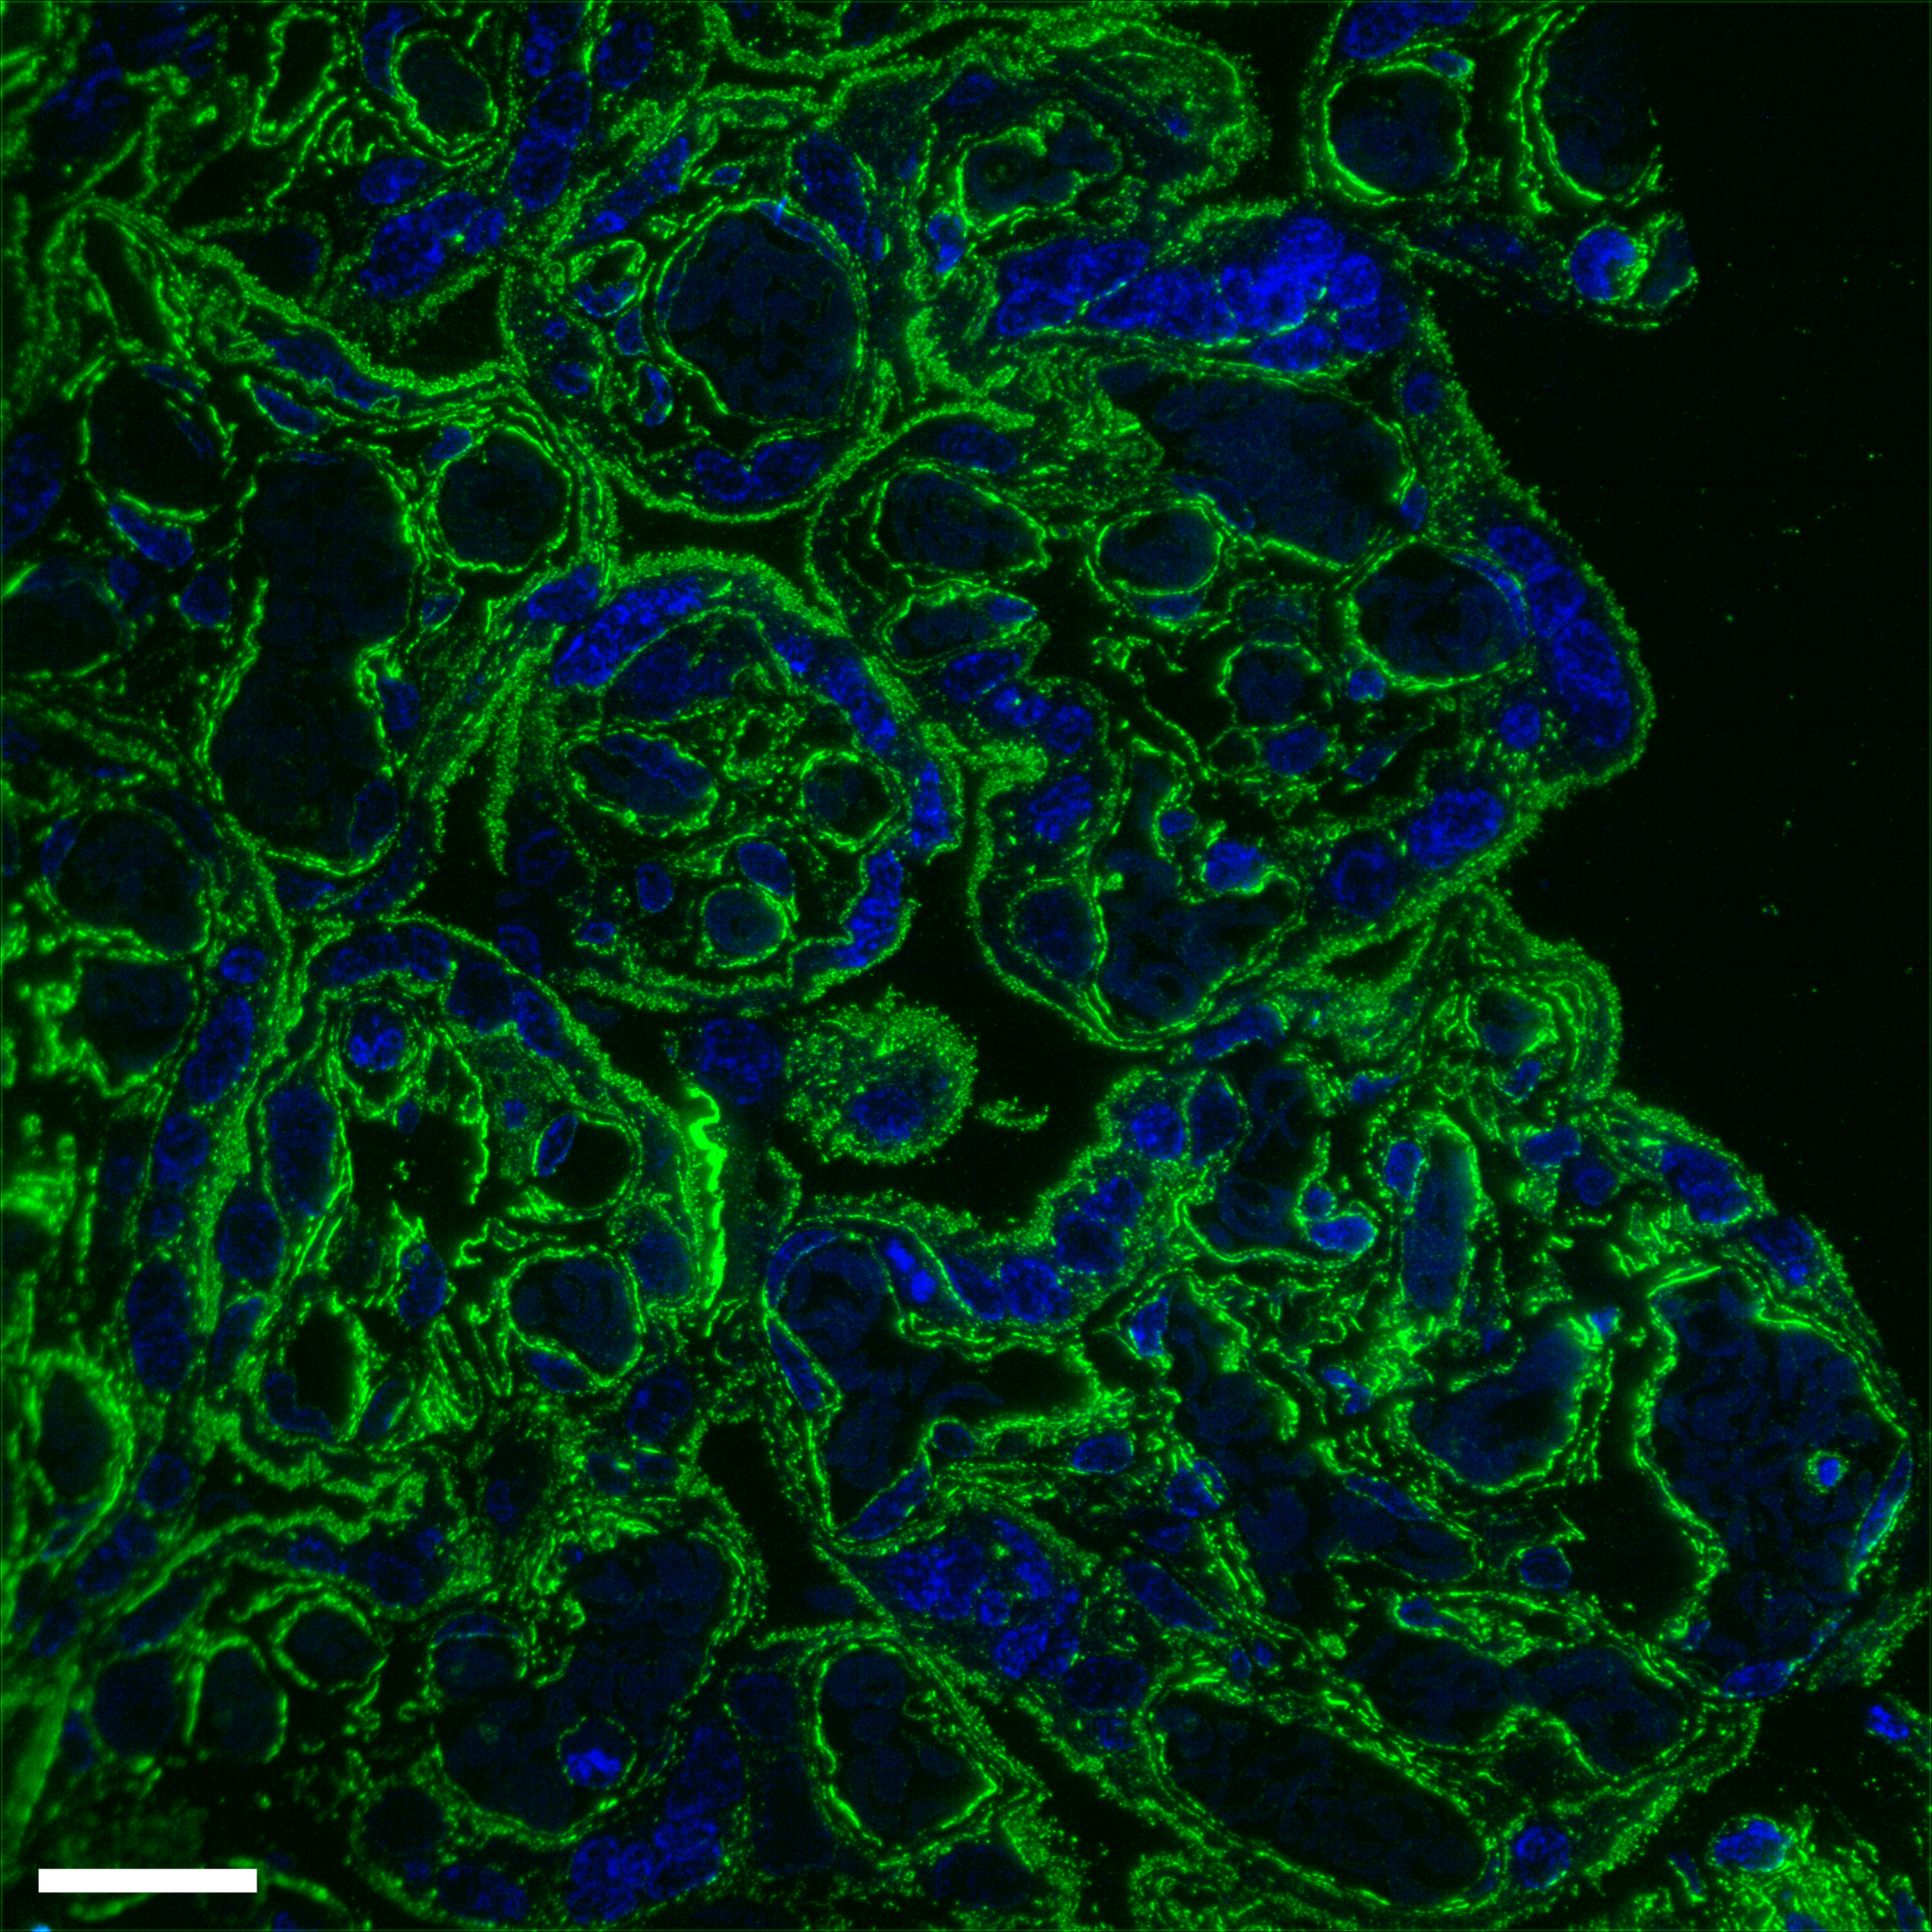}
%     \caption{This is a nanoscopy image of size 20000$\times$20000 pixels in 16 bit depth \cite{villegas2022chip} This nanoscopy image is from a single field-of-view of the microscope. In order to image a full biopsy sample for diagnosis and analysis purposes, several such consecutive regions are imaged and stitched together. Scale bar: 25 $\upmu$m.}
%     \label{fig:MUSICAL}
% \end{figure}

\section{UltraMNIST Dataset}

% to be uncommented later
%\input{neurips/app_plot_samples}

\section{UltraMNIST Dataset: Additional Details}

\subsection{Data documentation}

\subsection{Data acess for reviewers}

\subsection{Data hosting, licensing and maintenance}

\section{Unconstrained UltaMNIST classification}
\label{sec-ucons-umnist}

\section{Baseline Methods: Additional Details}
\subsection{Author statement}
\section{Appendix}

Include extra information in the appendix. This section will often be part of the supplemental material. Please see the call on the NeurIPS website for links to additional guides on dataset publication.

\begin{enumerate}

\item Submission introducing new datasets must include the following in the supplementary materials:
\begin{enumerate}
  \item Dataset documentation and intended uses. Recommended documentation frameworks include datasheets for datasets, dataset nutrition labels, data statements for NLP, and accountability frameworks.
  \item URL to website/platform where the dataset/benchmark can be viewed and downloaded by the reviewers.
  \item Author statement that they bear all responsibility in case of violation of rights, etc., and confirmation of the data license.
  \item Hosting, licensing, and maintenance plan. The choice of hosting platform is yours, as long as you ensure access to the data (possibly through a curated interface) and will provide the necessary maintenance.
\end{enumerate}

\item To ensure accessibility, the supplementary materials for datasets must include the following:
\begin{enumerate}
  \item Links to access the dataset and its metadata. This can be hidden upon submission if the dataset is not yet publicly available but must be added in the camera-ready version. In select cases, e.g when the data can only be released at a later date, this can be added afterward. Simulation environments should link to (open source) code repositories.
  \item The dataset itself should ideally use an open and widely used data format. Provide a detailed explanation on how the dataset can be read. For simulation environments, use existing frameworks or explain how they can be used.
  \item Long-term preservation: It must be clear that the dataset will be available for a long time, either by uploading to a data repository or by explaining how the authors themselves will ensure this.
  \item Explicit license: Authors must choose a license, ideally a CC license for datasets, or an open source license for code (e.g. RL environments).
  \item Add structured metadata to a dataset's meta-data page using Web standards (like schema.org and DCAT): This allows it to be discovered and organized by anyone. If you use an existing data repository, this is often done automatically.
  \item Highly recommended: a persistent dereferenceable identifier (e.g. a DOI minted by a data repository or a prefix on identifiers.org) for datasets, or a code repository (e.g. GitHub, GitLab,...) for code. If this is not possible or useful, please explain why.
\end{enumerate}

\item For benchmarks, the supplementary materials must ensure that all results are easily reproducible. Where possible, use a reproducibility framework such as the ML reproducibility checklist, or otherwise guarantee that all results can be easily reproduced, i.e. all necessary datasets, code, and evaluation procedures must be accessible and documented.

\item For papers introducing best practices in creating or curating datasets and benchmarks, the above supplementary materials are not required.
\end{enumerate}
